# Supplementary material for: Strain-driven superplasticity and modulation of electronic properties of ultrathin tin (II) oxide: A first-principles study
Source: arXiv:1911.04039 source file (2019-11-11)
Supplement: Supplementary file 1 [file Supplemental_Material.pdf]

# Supplemental Material

# Strain-driven superplasticity and modulation of electronic properties of ultrathin tin (II) oxide: A first-principles study

Devesh R. Kripalani,[1,2] Ping-Ping Sun,[1] Pamela Lin,[2] Ming Xue,[2] and Kun Zhou[1,*]

[1]*School of Mechanical and Aerospace Engineering,*
*Nanyang Technological University, Singapore 639798, Singapore*

[2]*Infineon Technologies Asia Pacific Pte Ltd, Singapore 349282, Singapore*

[*] kzhou@ntu.edu.sg

## I. ELASTIC CONSTANTS AND COMPRESSIBILITY CHARACTERIZATION

Under small deformations, for which Hooke's Law is valid, the mechanical properties of tin (II) oxide can be characterized based on its elastic constants. The deformation response $\boldsymbol{\epsilon}$ of a three-dimensional (3D) solid subject to a state of stress $\boldsymbol{\sigma}$ is described by the generalized stress-strain relation $\boldsymbol{\epsilon} = \mathbf{S}\boldsymbol{\sigma}$ (or equivalently $\boldsymbol{\sigma} = \mathbf{C}\boldsymbol{\epsilon}$, where $\mathbf{C} = \mathbf{S}^{-1}$), as shown in Eq. (S1). Here, $\mathbf{S}$ and $\mathbf{C}$ denote the compliance and stiffness matrices, respectively. They are $6 \times 6$ symmetric and contain the material-dependent elastic constants, namely the Young's modulus $E$, Poisson's ratio $\nu$ and shear modulus $G$. By convention, $\epsilon_i$ ($\sigma_i$) denotes the axial strain (stress) in the $i$ direction, while $\gamma_{ij}$ ($\tau_{ij}$) refers to the shear strain (stress) in the $ij$-plane.

$$\begin{bmatrix}\epsilon_x & \epsilon_y & \epsilon_z & \gamma_{yz} & \gamma_{xz} & \gamma_{xy}\end{bmatrix}^{\mathbf{T}} = \mathbf{S}\begin{bmatrix}\sigma_x & \sigma_y & \sigma_z & \tau_{yz} & \tau_{xz} & \tau_{xy}\end{bmatrix}^{\mathbf{T}} \tag{S1}$$

$$\text{where } \mathbf{S} = \begin{bmatrix} 1/E_x & -\nu_{yx}/E_y & -\nu_{zx}/E_z & 0 & 0 & 0 \\ -\nu_{xy}/E_x & 1/E_y & -\nu_{zy}/E_z & 0 & 0 & 0 \\ -\nu_{xz}/E_x & -\nu_{yz}/E_y & 1/E_z & 0 & 0 & 0 \\ 0 & 0 & 0 & 1/G_{yz} & 0 & 0 \\ 0 & 0 & 0 & 0 & 1/G_{xz} & 0 \\ 0 & 0 & 0 & 0 & 0 & 1/G_{xy} \end{bmatrix}$$

In the case of two-dimensional (2D) materials (e.g. $n$-layer SnO), plane stress conditions ($\sigma_z = \tau_{yz} = \tau_{xz} = 0$) are imposed due to free relaxation of the surface in the normal ($z$) direction. This leads to a simplified form for the stress-strain relation, given by Eq. (S2).

$$\begin{bmatrix}\epsilon_x \\ \epsilon_y \\ \gamma_{xy}\end{bmatrix} = \mathbf{S}\begin{bmatrix}\sigma_x \\ \sigma_y \\ \tau_{xy}\end{bmatrix}, \quad \epsilon_z = -\frac{\nu_{xz}}{E_x}\sigma_x - \frac{\nu_{yz}}{E_y}\sigma_y \tag{S2}$$

$$\text{where } \mathbf{S} = \begin{bmatrix} 1/E_x & -\nu_{yx}/E_y & 0 \\ -\nu_{xy}/E_x & 1/E_y & 0 \\ 0 & 0 & 1/G_{xy} \end{bmatrix}$$

To evaluate the elastic constants of tin (II) oxide, the potential energy surface of the system is first sampled under various strain configurations across the range -1.5% $\leq \epsilon_i \leq$ 1.5% and -3% $\leq \gamma_{ij} \leq$ 3%. In accordance with the linear theory of elasticity, the strain energy $E_\mathrm{s}$ stored in a material exhibits a quadratic dependence on the applied strains, as shown in Eqs. (S3) and (S4) for the general case (3D) and for prescribed plane stress conditions (2D), respectively. Here, $V_0$ and $A_0$ are the equilibrium volume and in-plane area of the simulation cell, while $t_0$ refers to the equilibrium thickness of $n$-layer SnO. By performing a fit to the strain energy surface, the stiffness matrix $\mathbf{C}$ of tin (II) oxide can be obtained, from which the elastic constants are subsequently derived.

$$E_\mathrm{s} = \frac{V_0}{2}\Big(C_{11}\epsilon_x^2 + C_{22}\epsilon_y^2 + C_{33}\epsilon_z^2 + 2C_{12}\epsilon_x\epsilon_y + 2C_{13}\epsilon_x\epsilon_z + 2C_{23}\epsilon_y\epsilon_z + C_{44}\gamma_{yz}^2 + C_{55}\gamma_{xz}^2 + C_{66}\gamma_{xy}^2\Big) \tag{S3}$$

$$E_\mathrm{s} = \frac{A_0 t_0}{2}\Big(C_{11}\epsilon_x^2 + C_{22}\epsilon_y^2 + 2C_{12}\epsilon_x\epsilon_y + C_{66}\gamma_{xy}^2\Big) \tag{S4}$$

The compressibility of bulk tin (II) oxide is characterized by the relations provided in Eq. (S5) under hydrostatic pressure conditions, where $\sigma_x = \sigma_y = \sigma_z = p$, and $\tau_{xy} = \tau_{yz} = \tau_{xz} = 0$. Accordingly, the bulk modulus $K$ provides a measure of the volumetric response to pressure, while the linear stiffness $B_\mathbf{u}$ in an arbitrary direction is defined along the unit vector $\mathbf{u} = l_1\mathbf{i} + l_2\mathbf{j} + l_3\mathbf{k}$, where $l_i$ are the direction cosines.

$$K = \left[\sum_{p=1}^{3}\sum_{q=1}^{3} S_{pq}\right]^{-1}, \quad B_\mathbf{u} = \left[\sum_{p=1}^{3}\left(\sum_{q=1}^{3} S_{pq}\right) l_p^2\right]^{-1} \tag{S5}$$

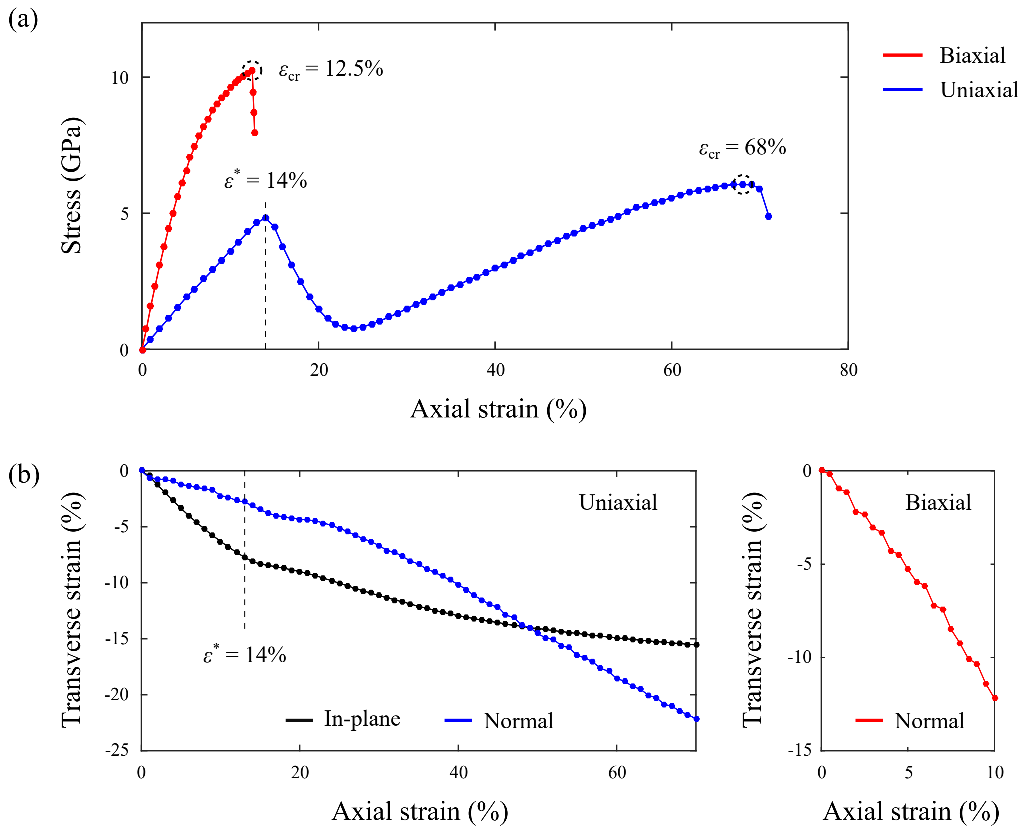


FIG. S1. (a) The stress-strain relationship, and (b) transverse relaxation response of bilayer SnO under applied biaxial and uniaxial strain conditions. The transition from low to high strain regimes in the uniaxial mode is denoted by dotted lines at $\epsilon^* = 14\%$.

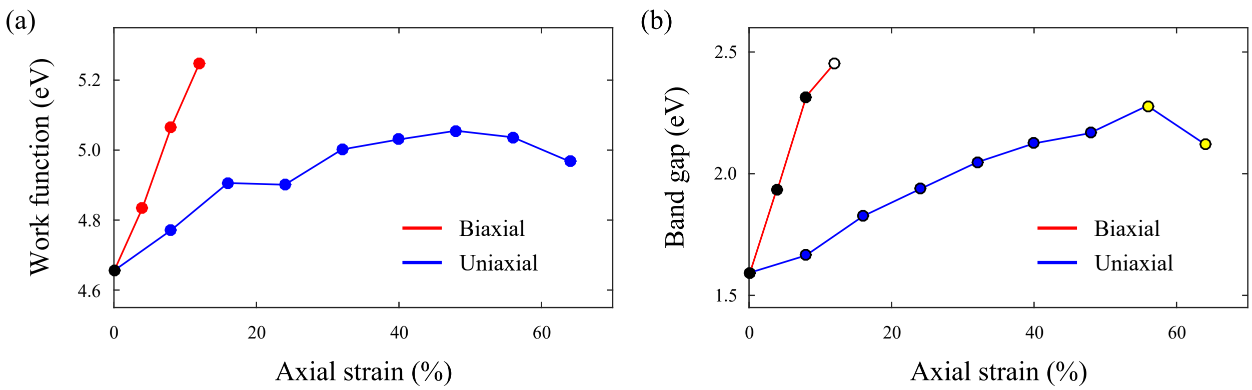


FIG. S2. The variation of the (a) work function, and (b) electronic band gap of bilayer SnO under applied biaxial and uniaxial strain conditions (Level of theory: HSE+D2). The VBM/CBM positions which make up the band gap are denoted by different colored markers according to the same definitions given in the main article (see Fig. 5(b)).
